# Supplementary material for: Reusable Slotwise Mechanisms
Source: arXiv:2302.10503 source file (2023-10-27)
Supplement: Supplementary file 1 [file reconstruct_Balls_appendix.tex]

\begin{figure}
  \centering
  \begin{tabular}{*{11}{@{\hspace{1px}}c}}
    Step= & 1 & 2 & 3 & 4 & 5 & 6 & 7 & 8 & 9 & 10 \\
    Groundtruth &
    \includegraphics[height=0.04\textheight]{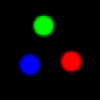} &
    \includegraphics[height=0.04\textheight]{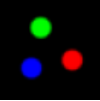} &
    \includegraphics[height=0.04\textheight]{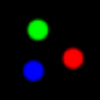} &
    \includegraphics[height=0.04\textheight]{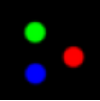} &
    \includegraphics[height=0.04\textheight]{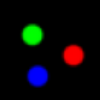} &
    \includegraphics[height=0.04\textheight]{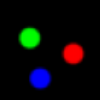} &
    \includegraphics[height=0.04\textheight]{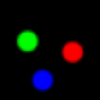} &
    \includegraphics[height=0.04\textheight]{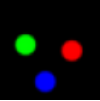} &
    \includegraphics[height=0.04\textheight]{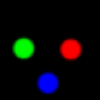} &
    \includegraphics[height=0.04\textheight]{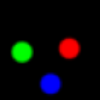} \\
    RSM (Ours) &
    \includegraphics[height=0.04\textheight]{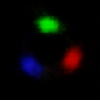} &
    \includegraphics[height=0.04\textheight]{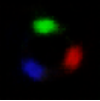} &
    \includegraphics[height=0.04\textheight]{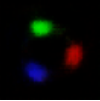} &
    \includegraphics[height=0.04\textheight]{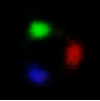} &
    \includegraphics[height=0.04\textheight]{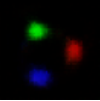} &
    \includegraphics[height=0.04\textheight]{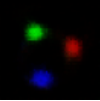} &
    \includegraphics[height=0.04\textheight]{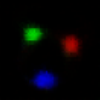} &
    \includegraphics[height=0.04\textheight]{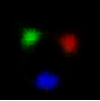} &
    \includegraphics[height=0.04\textheight]{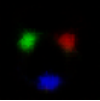} &
    \includegraphics[height=0.04\textheight]{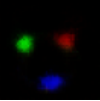} \\
    GNN &
    \includegraphics[height=0.04\textheight]{figures/reconstructed_imgs/IID/GNN/Balls/1_predictedx_1_test_GNN_medium_3_Ballsx10.pdf} &
    \includegraphics[height=0.04\textheight]{figures/reconstructed_imgs/IID/GNN/Balls/1_predictedx_2_test_GNN_medium_3_Ballsx10.pdf} &
    \includegraphics[height=0.04\textheight]{figures/reconstructed_imgs/IID/GNN/Balls/1_predictedx_3_test_GNN_medium_3_Ballsx10.pdf} &
    \includegraphics[height=0.04\textheight]{figures/reconstructed_imgs/IID/GNN/Balls/1_predictedx_4_test_GNN_medium_3_Ballsx10.pdf} &
    \includegraphics[height=0.04\textheight]{figures/reconstructed_imgs/IID/GNN/Balls/1_predictedx_5_test_GNN_medium_3_Ballsx10.pdf} &
    \includegraphics[height=0.04\textheight]{figures/reconstructed_imgs/IID/GNN/Balls/1_predictedx_6_test_GNN_medium_3_Ballsx10.pdf} &
    \includegraphics[height=0.04\textheight]{figures/reconstructed_imgs/IID/GNN/Balls/1_predictedx_7_test_GNN_medium_3_Ballsx10.pdf} &
    \includegraphics[height=0.04\textheight]{figures/reconstructed_imgs/IID/GNN/Balls/1_predictedx_8_test_GNN_medium_3_Ballsx10.pdf} &
    \includegraphics[height=0.04\textheight]{figures/reconstructed_imgs/IID/GNN/Balls/1_predictedx_9_test_GNN_medium_3_Ballsx10.pdf} &
    \includegraphics[height=0.04\textheight]{figures/reconstructed_imgs/IID/GNN/Balls/1_predictedx_10_test_GNN_medium_3_Ballsx10.pdf} \\
    MBRL &
    \includegraphics[height=0.04\textheight]{figures/reconstructed_imgs/IID/MBRL/Balls/1_predictedx_1_test_Modular_3_Balls_-1_-1_MLP_Ctxfalse10.pdf} &
    \includegraphics[height=0.04\textheight]{figures/reconstructed_imgs/IID/MBRL/Balls/1_predictedx_2_test_Modular_3_Balls_-1_-1_MLP_Ctxfalse10.pdf} &
    \includegraphics[height=0.04\textheight]{figures/reconstructed_imgs/IID/MBRL/Balls/1_predictedx_3_test_Modular_3_Balls_-1_-1_MLP_Ctxfalse10.pdf} &
    \includegraphics[height=0.04\textheight]{figures/reconstructed_imgs/IID/MBRL/Balls/1_predictedx_4_test_Modular_3_Balls_-1_-1_MLP_Ctxfalse10.pdf} &
    \includegraphics[height=0.04\textheight]{figures/reconstructed_imgs/IID/MBRL/Balls/1_predictedx_5_test_Modular_3_Balls_-1_-1_MLP_Ctxfalse10.pdf} &
    \includegraphics[height=0.04\textheight]{figures/reconstructed_imgs/IID/MBRL/Balls/1_predictedx_6_test_Modular_3_Balls_-1_-1_MLP_Ctxfalse10.pdf} &
    \includegraphics[height=0.04\textheight]{figures/reconstructed_imgs/IID/MBRL/Balls/1_predictedx_7_test_Modular_3_Balls_-1_-1_MLP_Ctxfalse10.pdf} &
    \includegraphics[height=0.04\textheight]{figures/reconstructed_imgs/IID/MBRL/Balls/1_predictedx_8_test_Modular_3_Balls_-1_-1_MLP_Ctxfalse10.pdf} &
    \includegraphics[height=0.04\textheight]{figures/reconstructed_imgs/IID/MBRL/Balls/1_predictedx_9_test_Modular_3_Balls_-1_-1_MLP_Ctxfalse10.pdf} &
    \includegraphics[height=0.04\textheight]{figures/reconstructed_imgs/IID/MBRL/Balls/1_predictedx_10_test_Modular_3_Balls_-1_-1_MLP_Ctxfalse10.pdf} \\
    NPS &
    \includegraphics[height=0.04\textheight]{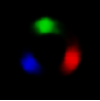} &
    \includegraphics[height=0.04\textheight]{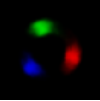} &
    \includegraphics[height=0.04\textheight]{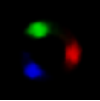} &
    \includegraphics[height=0.04\textheight]{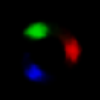} &
    \includegraphics[height=0.04\textheight]{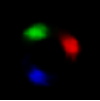} &
    \includegraphics[height=0.04\textheight]{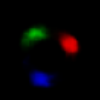} &
    \includegraphics[height=0.04\textheight]{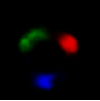} &
    \includegraphics[height=0.04\textheight]{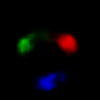} &
    \includegraphics[height=0.04\textheight]{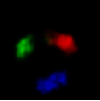} &
    \includegraphics[height=0.04\textheight]{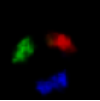} \\

  \end{tabular}
  \caption{Reconstruction comparison on 3-Body Physic dataset}
  \label{fig:recontruct_balls}
\end{figure}

\begin{figure}[t]
  \centering
  \begin{tabular}{*{8}{@{\hspace{1px}}c}}
    Step & Target & Predicted & Slot 1 & Slot 2 & Slot 3 \\
    RSM &
    \includegraphics[height=0.04\textheight]{figures/reconstructed_imgs/IID/Target/Balls/1_actual_4_test_Modular_medium_3_Ballsx_7_5_xrandom10.pdf} &
    \includegraphics[height=0.04\textheight]{figures/reconstructed_imgs/IID/RSM/Balls_2/1_predicted_4_test_Modular_3_Balls_3_5_attn_Ctxtrue10.pdf} &
    \includegraphics[height=0.04\textheight]{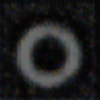} &
    \includegraphics[height=0.04\textheight]{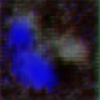} &
    \includegraphics[height=0.04\textheight]{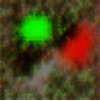} \\
    % RSM ab par &
    %     \includegraphics[height=0.04\textheight]{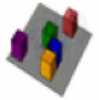} &
    
    % \includegraphics[height=0.04\textheight]{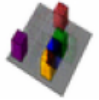} &
    % \includegraphics[height=0.04\textheight]{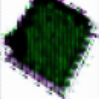} &
    % \includegraphics[height=0.04\textheight]{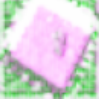} &
    % \includegraphics[height=0.04\textheight]{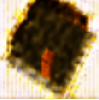} &
    % \includegraphics[height=0.04\textheight]{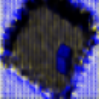} &
    % \includegraphics[height=0.04\textheight]{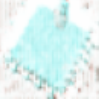} \\
    MBRL &
    \includegraphics[height=0.04\textheight]{figures/reconstructed_imgs/IID/Target/Balls/1_actual_4_test_Modular_medium_3_Ballsx_7_5_xrandom10.pdf} &
    \includegraphics[height=0.04\textheight]{figures/reconstructed_imgs/IID/MBRL/Balls/1_predictedx_5_test_Modular_3_Balls_-1_-1_MLP_Ctxfalse10.pdf} &
    \includegraphics[height=0.04\textheight]{figures/reconstructed_imgs/IID/MBRL/Balls/1_slot0_4_test_Modular_medium_3_Balls_-1_-1_xrandom10.pdf} &
    \includegraphics[height=0.04\textheight]{figures/reconstructed_imgs/IID/MBRL/Balls/1_slot1_4_test_Modular_medium_3_Balls_-1_-1_xrandom10.pdf} &
    \includegraphics[height=0.04\textheight]{figures/reconstructed_imgs/IID/MBRL/Balls/1_slot2_4_test_Modular_medium_3_Balls_-1_-1_xrandom10.pdf} \\
    NPS &
    \includegraphics[height=0.04\textheight]{figures/reconstructed_imgs/IID/Target/Balls/1_actual_4_test_Modular_medium_3_Ballsx_7_5_xrandom10.pdf} &
    \includegraphics[height=0.04\textheight]{figures/reconstructed_imgs/IID/NPS/Balls/1_predicted_4_test_Balls_NPS.pdf} &
    \includegraphics[height=0.04\textheight]{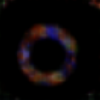} &
    \includegraphics[height=0.04\textheight]{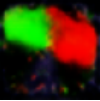} &
    \includegraphics[height=0.04\textheight]{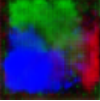} \\
  \end{tabular}
  \caption{Comparison of the decoded slots at step 5 in the Balls environment}
  \label{fig:reconstruct_slots_balls}
\end{figure}
