# Supplementary material for: Reusable Slotwise Mechanisms
Source: arXiv:2302.10503 source file (2023-10-27)
Supplement: Supplementary file 2 [file reconstruct_Breakout_appendix.tex]

\begin{figure}
  \centering
  \begin{tabular}{*{11}{@{\hspace{1px}}c}}
    Step= & 1 & 2 & 3 & 4 & 5 & 6 & 7 & 8 & 9 & 10 \\
    Groundtruth &
    \includegraphics[height=0.04\textheight]{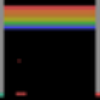} &
    \includegraphics[height=0.04\textheight]{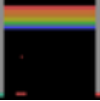} &
    \includegraphics[height=0.04\textheight]{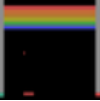} &
    \includegraphics[height=0.04\textheight]{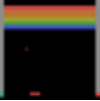} &
    \includegraphics[height=0.04\textheight]{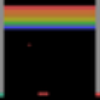} &
    \includegraphics[height=0.04\textheight]{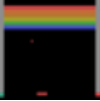} &
    \includegraphics[height=0.04\textheight]{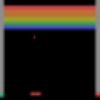} &
    \includegraphics[height=0.04\textheight]{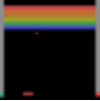} &
    \includegraphics[height=0.04\textheight]{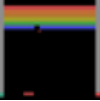} &
    \includegraphics[height=0.04\textheight]{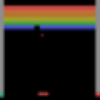} \\
    RSM (Ours) &
    \includegraphics[height=0.04\textheight]{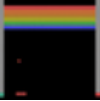} &
    \includegraphics[height=0.04\textheight]{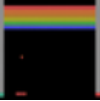} &
    \includegraphics[height=0.04\textheight]{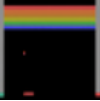} &
    \includegraphics[height=0.04\textheight]{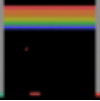} &
    \includegraphics[height=0.04\textheight]{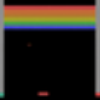} &
    \includegraphics[height=0.04\textheight]{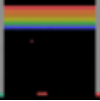} &
    \includegraphics[height=0.04\textheight]{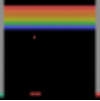} &
    \includegraphics[height=0.04\textheight]{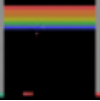} &
    \includegraphics[height=0.04\textheight]{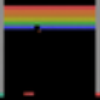} &
    \includegraphics[height=0.04\textheight]{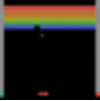} \\
    GNN &
    \includegraphics[height=0.04\textheight]{figures/reconstructed_imgs/IID/GNN/Breakout/0_predicted_0_test_GNN_medium_3_Breakout10.pdf} &
    \includegraphics[height=0.04\textheight]{figures/reconstructed_imgs/IID/GNN/Breakout/0_predicted_1_test_GNN_medium_3_Breakout10.pdf} &
    \includegraphics[height=0.04\textheight]{figures/reconstructed_imgs/IID/GNN/Breakout/0_predicted_2_test_GNN_medium_3_Breakout10.pdf} &
    \includegraphics[height=0.04\textheight]{figures/reconstructed_imgs/IID/GNN/Breakout/0_predicted_3_test_GNN_medium_3_Breakout10.pdf} &
    \includegraphics[height=0.04\textheight]{figures/reconstructed_imgs/IID/GNN/Breakout/0_predicted_4_test_GNN_medium_3_Breakout10.pdf} &
    \includegraphics[height=0.04\textheight]{figures/reconstructed_imgs/IID/GNN/Breakout/0_predicted_5_test_GNN_medium_3_Breakout10.pdf} &
    \includegraphics[height=0.04\textheight]{figures/reconstructed_imgs/IID/GNN/Breakout/0_predicted_6_test_GNN_medium_3_Breakout10.pdf} &
    \includegraphics[height=0.04\textheight]{figures/reconstructed_imgs/IID/GNN/Breakout/0_predicted_7_test_GNN_medium_3_Breakout10.pdf} &
    \includegraphics[height=0.04\textheight]{figures/reconstructed_imgs/IID/GNN/Breakout/0_predicted_8_test_GNN_medium_3_Breakout10.pdf} &
    \includegraphics[height=0.04\textheight]{figures/reconstructed_imgs/IID/GNN/Breakout/0_predicted_9_test_GNN_medium_3_Breakout10.pdf} \\
    MBRL &
    \includegraphics[height=0.04\textheight]{figures/reconstructed_imgs/IID/MBRL/Breakout/0_predicted_0_test_Modular_medium_3_Breakout_-1_-1_xrandom10.pdf} &
    \includegraphics[height=0.04\textheight]{figures/reconstructed_imgs/IID/MBRL/Breakout/0_predicted_1_test_Modular_medium_3_Breakout_-1_-1_xrandom10.pdf} &
    \includegraphics[height=0.04\textheight]{figures/reconstructed_imgs/IID/MBRL/Breakout/0_predicted_2_test_Modular_medium_3_Breakout_-1_-1_xrandom10.pdf} &
    \includegraphics[height=0.04\textheight]{figures/reconstructed_imgs/IID/MBRL/Breakout/0_predicted_3_test_Modular_medium_3_Breakout_-1_-1_xrandom10.pdf} &
    \includegraphics[height=0.04\textheight]{figures/reconstructed_imgs/IID/MBRL/Breakout/0_predicted_4_test_Modular_medium_3_Breakout_-1_-1_xrandom10.pdf} &
    \includegraphics[height=0.04\textheight]{figures/reconstructed_imgs/IID/MBRL/Breakout/0_predicted_5_test_Modular_medium_3_Breakout_-1_-1_xrandom10.pdf} &
    \includegraphics[height=0.04\textheight]{figures/reconstructed_imgs/IID/MBRL/Breakout/0_predicted_6_test_Modular_medium_3_Breakout_-1_-1_xrandom10.pdf} &
    \includegraphics[height=0.04\textheight]{figures/reconstructed_imgs/IID/MBRL/Breakout/0_predicted_7_test_Modular_medium_3_Breakout_-1_-1_xrandom10.pdf} &
    \includegraphics[height=0.04\textheight]{figures/reconstructed_imgs/IID/MBRL/Breakout/0_predicted_8_test_Modular_medium_3_Breakout_-1_-1_xrandom10.pdf} &
    \includegraphics[height=0.04\textheight]{figures/reconstructed_imgs/IID/MBRL/Breakout/0_predicted_9_test_Modular_medium_3_Breakout_-1_-1_xrandom10.pdf} \\
    NPS &
    \includegraphics[height=0.04\textheight]{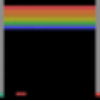} &
    \includegraphics[height=0.04\textheight]{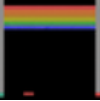} &
    \includegraphics[height=0.04\textheight]{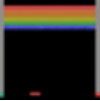} &
    \includegraphics[height=0.04\textheight]{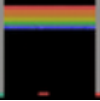} &
    \includegraphics[height=0.04\textheight]{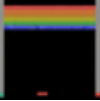} &
    \includegraphics[height=0.04\textheight]{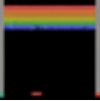} &
    \includegraphics[height=0.04\textheight]{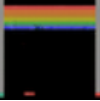} &
    \includegraphics[height=0.04\textheight]{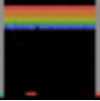} &
    \includegraphics[height=0.04\textheight]{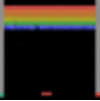} &
    \includegraphics[height=0.04\textheight]{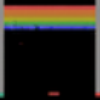} \\

  \end{tabular}
  \caption{Reconstruction comparison on Breakout dataset}
  \label{fig:reconstruct_breakout}
\end{figure}
