# Supplementary material for: Reusable Slotwise Mechanisms
Source: arXiv:2302.10503 source file (2023-10-27)
Supplement: Supplementary file 4 [file reconstruct_Shapes_appendix.tex]

\begin{figure}
  \centering
  \begin{tabular}{*{7}{@{\hspace{0px}}c}}
     & \multicolumn{1}{c}{Input} & \multicolumn{5}{c}{Extracted feature maps} \\
    RSM & \multicolumn{6}{c}{\includegraphics[height=0.04\textheight]{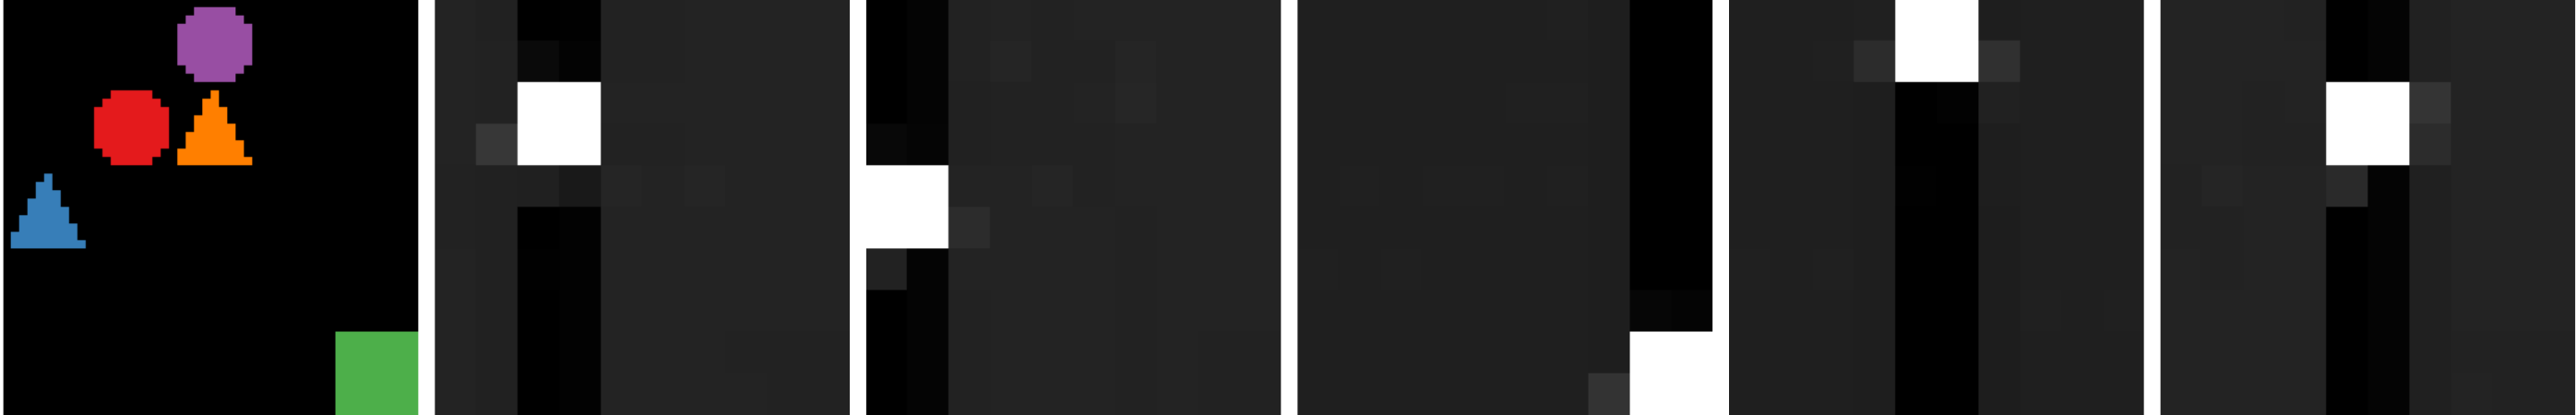}}\\
    MBRL & \multicolumn{6}{c}{\includegraphics[height=0.04\textheight]{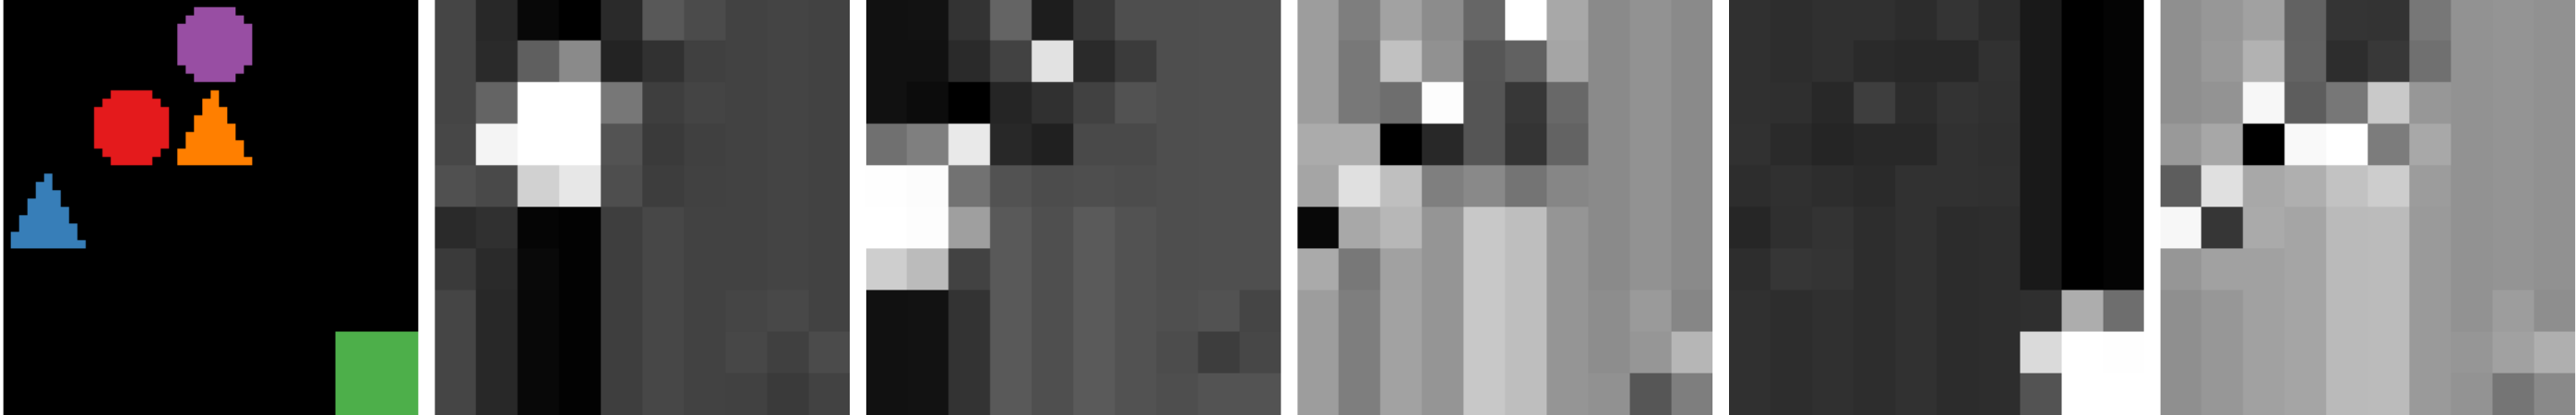}}\\
    NPS & \multicolumn{6}{c}{\includegraphics[height=0.04\textheight]{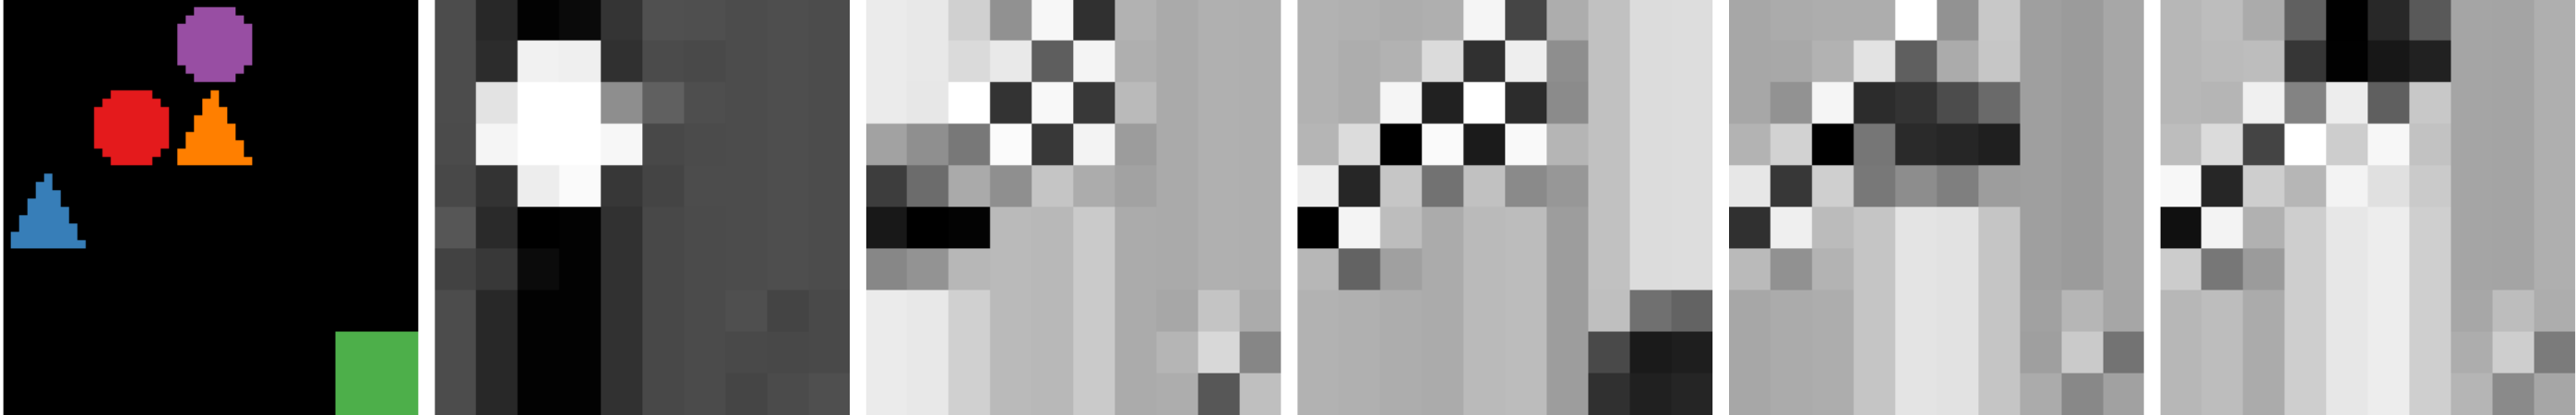}}\\
  \end{tabular}
  \caption{Comparison of extracted feature maps from a scene in 2D Shapes environment}
  \label{fig:feature_maps_2d}
\end{figure}

\begin{figure}
  \centering
  \begin{tabular}{*{11}{@{\hspace{1px}}c}}
    Step= & 1 & 2 & 3 & 4 & 5 & 6 & 7 & 8 & 9 & 10 \\
    Groundtruth &
    \includegraphics[height=0.04\textheight]{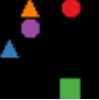} &
    \includegraphics[height=0.04\textheight]{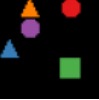} &
    \includegraphics[height=0.04\textheight]{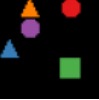} &
    \includegraphics[height=0.04\textheight]{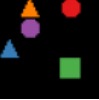} &
    \includegraphics[height=0.04\textheight]{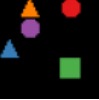} &
    \includegraphics[height=0.04\textheight]{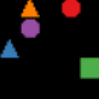} &
    \includegraphics[height=0.04\textheight]{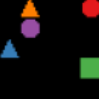} &
    \includegraphics[height=0.04\textheight]{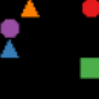} &
    \includegraphics[height=0.04\textheight]{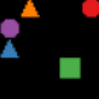} &
    \includegraphics[height=0.04\textheight]{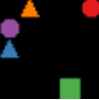} \\
    RSM &
    \includegraphics[height=0.04\textheight]{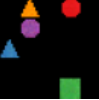} &
    \includegraphics[height=0.04\textheight]{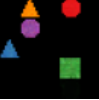} &
    \includegraphics[height=0.04\textheight]{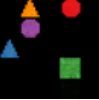} &
    \includegraphics[height=0.04\textheight]{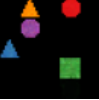} &
    \includegraphics[height=0.04\textheight]{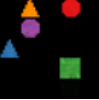} &
    \includegraphics[height=0.04\textheight]{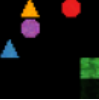} &
    \includegraphics[height=0.04\textheight]{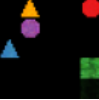} &
    \includegraphics[height=0.04\textheight]{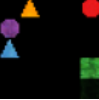} &
    \includegraphics[height=0.04\textheight]{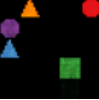} &
    \includegraphics[height=0.04\textheight]{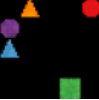} \\
    GNN &
    \includegraphics[height=0.04\textheight]{figures/reconstructed_imgs/IID/GNN/Shapes/7_predicted_1_test_GNN_5_Shapes10.pdf} &
    \includegraphics[height=0.04\textheight]{figures/reconstructed_imgs/IID/GNN/Shapes/7_predicted_2_test_GNN_5_Shapes10.pdf} &
    \includegraphics[height=0.04\textheight]{figures/reconstructed_imgs/IID/GNN/Shapes/7_predicted_3_test_GNN_5_Shapes10.pdf} &
    \includegraphics[height=0.04\textheight]{figures/reconstructed_imgs/IID/GNN/Shapes/7_predicted_4_test_GNN_5_Shapes10.pdf} &
    \includegraphics[height=0.04\textheight]{figures/reconstructed_imgs/IID/GNN/Shapes/7_predicted_5_test_GNN_5_Shapes10.pdf} &
    \includegraphics[height=0.04\textheight]{figures/reconstructed_imgs/IID/GNN/Shapes/7_predicted_6_test_GNN_5_Shapes10.pdf} &
    \includegraphics[height=0.04\textheight]{figures/reconstructed_imgs/IID/GNN/Shapes/7_predicted_7_test_GNN_5_Shapes10.pdf} &
    \includegraphics[height=0.04\textheight]{figures/reconstructed_imgs/IID/GNN/Shapes/7_predicted_8_test_GNN_5_Shapes10.pdf} &
    \includegraphics[height=0.04\textheight]{figures/reconstructed_imgs/IID/GNN/Shapes/7_predicted_9_test_GNN_5_Shapes10.pdf} &
    \includegraphics[height=0.04\textheight]{figures/reconstructed_imgs/IID/GNN/Shapes/7_predicted_10_test_GNN_5_Shapes10.pdf} \\
    MBRL &
    \includegraphics[height=0.04\textheight]{figures/reconstructed_imgs/IID/MBRL/Shapes/7_predicted_1_test_Modular_5_Shapes_-1_-1_MLP_Ctxfalse10.pdf} &
    \includegraphics[height=0.04\textheight]{figures/reconstructed_imgs/IID/MBRL/Shapes/7_predicted_2_test_Modular_5_Shapes_-1_-1_MLP_Ctxfalse10.pdf} &
    \includegraphics[height=0.04\textheight]{figures/reconstructed_imgs/IID/MBRL/Shapes/7_predicted_3_test_Modular_5_Shapes_-1_-1_MLP_Ctxfalse10.pdf} &
    \includegraphics[height=0.04\textheight]{figures/reconstructed_imgs/IID/MBRL/Shapes/7_predicted_4_test_Modular_5_Shapes_-1_-1_MLP_Ctxfalse10.pdf} &
    \includegraphics[height=0.04\textheight]{figures/reconstructed_imgs/IID/MBRL/Shapes/7_predicted_5_test_Modular_5_Shapes_-1_-1_MLP_Ctxfalse10.pdf} &
    \includegraphics[height=0.04\textheight]{figures/reconstructed_imgs/IID/MBRL/Shapes/7_predicted_6_test_Modular_5_Shapes_-1_-1_MLP_Ctxfalse10.pdf} &
    \includegraphics[height=0.04\textheight]{figures/reconstructed_imgs/IID/MBRL/Shapes/7_predicted_7_test_Modular_5_Shapes_-1_-1_MLP_Ctxfalse10.pdf} &
    \includegraphics[height=0.04\textheight]{figures/reconstructed_imgs/IID/MBRL/Shapes/7_predicted_8_test_Modular_5_Shapes_-1_-1_MLP_Ctxfalse10.pdf} &
    \includegraphics[height=0.04\textheight]{figures/reconstructed_imgs/IID/MBRL/Shapes/7_predicted_9_test_Modular_5_Shapes_-1_-1_MLP_Ctxfalse10.pdf} &
    \includegraphics[height=0.04\textheight]{figures/reconstructed_imgs/IID/MBRL/Shapes/7_predicted_10_test_Modular_5_Shapes_-1_-1_MLP_Ctxfalse10.pdf} \\
    NPS &
    \includegraphics[height=0.04\textheight]{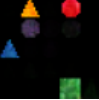} &
    \includegraphics[height=0.04\textheight]{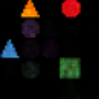} &
    \includegraphics[height=0.04\textheight]{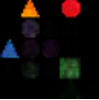} &
    \includegraphics[height=0.04\textheight]{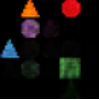} &
    \includegraphics[height=0.04\textheight]{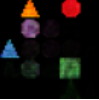} &
    \includegraphics[height=0.04\textheight]{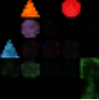} &
    \includegraphics[height=0.04\textheight]{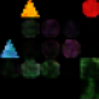} &
    \includegraphics[height=0.04\textheight]{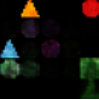} &
    \includegraphics[height=0.04\textheight]{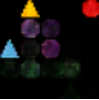} &
    \includegraphics[height=0.04\textheight]{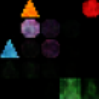} \\

  \end{tabular}
  \caption{Reconstruction comparison on 2D Shapes dataset}
  \label{fig:reconstruct_shapes}
\end{figure}
